# Supplementary material for: SADAS: A Dialogue Assistant System Towards Remediating Norm Violations in Bilingual Socio-Cultural Conversations
Source: arXiv:2402.01736 source file (2024-01-29)
Supplement: Supplementary file 1 [file 9-appendix.tex]

\appendix

\section{Example Appendix}
\label{sec:appendix}

This is an appendix.
